# Supplementary material for: A Disruptive Research Playbook for Studying Disruptive Innovations
Source: arXiv:2402.13329 source file (2024-02-20)
Supplement: Supplementary file 1 [file appendix-oldstuff.tex]

\appendix{Old stuff}

% may integrate in the framework section?)
\begin{itemize}
\item Defining and refining the \textbf{research questions}: 
    \begin{itemize}
        \item which \textbf{dimensions/phenomena} to consider and from which concern of \textbf{McLuhan's tetrad} to consider for each possible dimension?
    \end{itemize}
\item Designing the \textbf{research study/methodology}:
    \begin{itemize}
        \item which \textbf{theories} may be relevant - that we can build on for research study design or analysis
        \item which \textbf{research method(s)} should be used as guided by the research questions, dimensions, theories and pragmatic concerns
    \end{itemize}
\end{itemize}

% maybe integrate in AI section?
Typically, when a new ``solution'' that leverages AI is proposed, it is often with a specific benefit or advantage in mind that is driven by a specific problem that needs to be solved. For example, a bot that automates code review may be motivated by the need to reduce the work of developers and improve the quality of the code. A top of mind evaluation of this bot may measure the amount of developer time saved from doing code reviews or it may count the number of bugs it helps avoid. But such an evaluation would not account for other effects this bot may have on, for example on  knowledge diffusion across a team over time~\cite{Pascarella:etAl:2018} or on developer satisfaction who lose the chance to help others~\cite{storey}.  Broadening the questions asked by or goals behind a research study, is not a simple task.  

% may integrate some of this in the conceptual domain part of the framework
\subsection{Theories -- Daniel }

\textbf{Social Cognitive Theory:} This theory emphasizes the role of observational learning, self-efficacy, and motivation in human behavior. In the context of onboarding new contributors to Open Source projects, this theory suggests that providing access to LLMs could help new contributors learn by observing the behavior of experienced contributors, increase their self-efficacy by giving them a sense of mastery over the material, and increase their motivation by making the learning process more engaging.

\textbf{Cognitive Load Theory:} This theory posits that the working memory has a limited capacity, and that cognitive load can be managed through the use of instructional design strategies that reduce extraneous cognitive load and increase germane cognitive load. In the context of onboarding new contributors to Open Source projects, this theory suggests that using LLMs could help manage cognitive load by providing a structured and interactive learning experience that reduces the need for learners to remember and organize information on their own.

\textbf{Self-Determination Theory:} This theory emphasizes the importance of autonomy, competence, and relatedness in promoting intrinsic motivation and positive outcomes. In the context of onboarding new contributors to Open Source projects, this theory suggests that providing access to LLMs could increase the autonomy of new contributors by giving them more control over their learning process, increase their sense of competence by providing them with a structured and effective learning experience, and increase their sense of relatedness by connecting them to the community of contributors.

\textbf{Social Learning Theory:} This theory emphasizes the role of social interactions in learning, and suggests that learning occurs through observation, imitation, and reinforcement. In the context of onboarding new contributors to Open Source projects, this theory suggests that providing access to LLMs could facilitate social learning by giving new contributors access to examples of good practice, opportunities to observe and imitate experienced contributors, and feedback on their performance.

\textbf{Flow Theory:} This theory posits that people are most engaged and effective when they are in a state of flow, characterized by intense focus, a sense of control, and a feeling of enjoyment. In the context of onboarding new contributors to Open Source projects, this theory suggests that using LLMs could help new contributors achieve a state of flow by providing a challenging and rewarding learning experience that is tailored to their level of expertise and interests.

% not sure we need this anymore - could be too much detail but could mention the unit of analysis as a concept in the discussion perhaps?
\subsubsection{Unit of Analysis}

The research goals inherently suggest the phenomena under investigation. For instance, a study may explore the effect of team diversity on software development outcomes [ADD EXAMPLE RELATED TO THE PAPER]. In essence, this pertains to the 'unit of analysis,' which typically denotes the principal entity or subject examined, measured, and analyzed in a given research project~\cite{babbie2020}. The significance of clearly identifying the unit of analysis lies in its crucial role in influencing the selection of suitable methods and interpreting results~\cite{kozlowski2000multilevel}.

The accurate identification of the unit of analysis is vital for at least three primary reasons:

\begin{enumerate}
\item \textbf{Ensuring validity}: Choosing the appropriate unit of analysis guarantees that research findings accurately represent the relationships under study and are valid~\cite{yin2014}. Incorrect or mismatched units of analysis can result in errors in study design, data collection, and results interpretation, ultimately compromising the research's validity.
\item \textbf{Facilitating comparison and generalization}: By explicitly identifying and standardizing units of analysis, researchers can more readily compare results across various studies, facilitating a better understanding of trends and patterns in the field~\cite{george2005}. Moreover, maintaining a consistent unit of analysis enables generalizations, contributing to the development of more comprehensive theories.
\item \textbf{Guiding the choice of methodology}: The unit of analysis informs the selection of research methods and data collection techniques, ensuring alignment with the research question and objectives~\cite{eisenhardt2007theory}. A discrepancy between the unit of analysis and the chosen methodology can yield inaccurate or inconclusive findings.
\end{enumerate}

Thus far, software engineering research has employed an extensive range of units of analysis, reflecting the field's diverse research questions and objectives. Typical examples include:

... we had the various units here ... already integrated in the current version of the paper

The units of analysis presented in this section serve as examples and are by no means exhaustive. It is possible for researchers to adopt more than one unit of analysis in their work or explore new perspectives. Nevertheless, it remains crucial to explicitly state and address the chosen units of analysis in order to ensure validity, facilitate comparison and generalization, and guide methodological choices. By clearly identifying the units of analysis and acknowledging their implications, researchers can enhance the rigor of their studies and contribute to the advancement of the software engineering field.

% I think we don't need this but copying here
\begin{itemize}
    \item Quality (bug, vulnerability, software waste – lots of this)
    \item Speed/velocity of work (performance, we see lots of this)
    \item Individual Developer Experience (cognitive load/fatigue/processes/\\
    behaviours/values/flow, onboarding/learning, etc)
    \item Team (communication, coordination 
   knowledge/idea flow, culture, organizational behaviour/change)
    \item Organization (processes, economics)
    \item Societal (human values, ethics, privacy, intellectual property, sustainability)
    \item Professional (who is a software engineer, change in roles/expectations)
    \item Technological innovations
    \item Research community / directions /values (e.g., ethical reflection)
\end{itemize}

% our second two scenarios from our earlier version of the paper - maybe keep or put in an appendix or something - or online as examples of how o use the framework?

We consider three scenarios that vary according to their position on a socio-technical continuum.  We mention the more technical examples first to emphasize that even for those cases, human and social aspects should usually be considered. 

\begin{itemize}
    \item Using LLMs to enhance \textbf{automated program repair} (more technical than social, but there are less obvious impacts on human aspects such as adoption of the automation)  Humans supervise AI 
    % todo: ask Mark Harman which of his papers he discusses where the developers "steal" ideas from APR as their own work - maybe we want to touch on ethics?
    \item Using LLMs to support the \textbf{code review} process (social and technical aspects to consider - AI supervises the humans?
    \item Using LLMs to enhance the \textbf{onboarding} experience for new developers (more social than technical, but some technical concerns may be important too such as impact of early contributions on the quality of the code) Augmenting the humans through AI.
\end{itemize}

\subsection{LLMs and Code Review - Dong \& Takashi}
\dong{Code review is widely regarded as a cornerstone for software quality assurance. -- we could discuss the dimensions from the perspective of product (code quality), human (reviewers, authors), and process (review process).
\begin{itemize}
    \item \ul{RQ1: Impact on automated code review activities (Enhance).} defect prediction, code transformations (contributor), review comment generation (reviewer) 
    \item \ul{RQ2: Impact on the consumption of energy (e.g., carbon footprint) and finance (Retrieve).} Software waste \url{https://english.elpais.com/science-tech/2023-03-23/the-dirty-secret-of-artificial-intelligence.html}
    \item \ul{RQ3: Impact on code quality (Reverse).} security/vulnerability/copyright 
    \item \ul{RQ4: Impact on reviewer participation (Obsolete).} necessity of reviewer recommendation
    \item \ul{RQ5: Impact on review efficiency.} divergent review scores/review conflicts/knowledge transfer
\end{itemize}
}

\dong{unsure about ``retrieve'' aspect.}

\dong{Three latest systematic mapping studies that provide the existing CR themes: (i) Modern Code Reviews - A Survey of Literature and Practice, (ii) Can We Benchmark Code Review Studies?, and (iii) A Systematic Literature Review and Taxonomy of Modern Code Review.}

\subsection{LLMs and Onboarding - Dong}
\dong{Keeping a good influx of new contributors is critical for the project's survival and long-term success~\cite{rehman2022newcomer}.
With the wide adoption of large language models in the future, we assume that such adoption would reshape the onboarding process.
% :  (refine our question based on the problem that was to be solved and clarify what is it we want to know/learn).
Specifically, we could ask the following research questions for example by referring to McLuhan's framework:
\begin{itemize}
    \item \ul{RQ1: Impact on the code quality by newcomers (Enhance).}
    \item \ul{RQ2: Impact on knowledge transferring within a team (Reverse).} \citet{Scacchi2002IEE} found that newcomers in OSS projects are usually expected to learn about the project on their own. Similarly, \citet{rehman2022newcomer} empirically observed that after joining GitHub, the majority of newcomers are less likely to do social coding in terms of commits and pull requests. One of the advantages of the social platforms (e.g., GitHub) is to share and transfer knowledge. We hypothesize that the emergency of LLMs would further decrease the probability of learning among developers' collaboration.
    \item \ul{RQ3: Impact on the barriers faced by newcomers (Obsolete and Reverse).} Prior work pointed out that newcomers face several barriers to onboarding open-source projects, such as finding a way to start, technical hurdles, and social interaction~\cite{igor2014IST}. 
    Explicitly, newcomers to a project, send contributions that are not incorporated into the code base and give up contributing~\cite{Igor2015CSCW}.
    We hypothesize that on the one hand, the adoption of LLMs
    would lower the barrier for newcomers to onboard as the LLMs is possible to suggest codes.
    On the other hand, it may introduce new barriers. 
    For instance, the codes contributed by the newcomers would be of low quality without taking into account the project's code guidelines.
    \item \ul{RQ4: Impact on the social environment (Reverse).} \citet{igor2014IST} also highlighted that toxicity might impair effective collaboration and prevent newcomers from contributing to open-source projects.
    The willingness of individual and project’s climate were associated with the odds that an individual would become a long-term contributor~\cite{Zhou2015TSE}.
    We hypothesize that the adoption of LLMs may incur a toxic collaboration environment. Although the LLMs possibly reduce the human interaction between developers, the quality of contributions would bring confusion and reversely may cause a conflict.
\end{itemize}}
Possible dimensions (and thus questions) to consider? 
% -> RQ1:  Impact on new contributors’ learning (individual, enhance)
-> RQ2:  Impact on team expertise (team, reverse)
Impact on speed and cost of onboarding new developers (organization, enhance) 
Impact on quality of the code by new contributors (quality, enhance)
Impact on toxicity during onboarding (society, reverse)
Will LLMs lower the barriers change who contributes to and how (profession, obsolete)
