# Supplementary material for: A Disruptive Research Playbook for Studying Disruptive Innovations
Source: arXiv:2402.13329 source file (2024-02-20)
Supplement: Supplementary file 2 [file appendix-theories.tex]

\appendix{Theories}

Courtesy of ChatGPT

\subsection*{What theories can we use for understanding code review in software development}

Code review is an important process in software development that involves examining code written by one or more developers to identify errors, improve the quality of the code, and ensure that it meets the project's requirements. Here are some theories that can be used to understand code review in software development:

Cognitive Load Theory: Cognitive Load Theory suggests that the human brain can only process a limited amount of information at a time. In code review, this means that reviewers can only process a certain amount of code at a time before their cognitive load becomes too high, and they start to miss errors. Understanding the limitations of cognitive load can help teams to structure code reviews in a way that is manageable and effective.

Social Learning Theory: Social Learning Theory emphasizes the importance of learning through observation and interaction with others. In code review, this means that the process of reviewing code can help team members learn from each other and improve their skills. By providing feedback and guidance, reviewers can help developers to learn new techniques and best practices.

Information Processing Theory: Information Processing Theory suggests that humans process information in stages, starting with sensory input and moving through various levels of processing before generating a response. In code review, this means that reviewers must first identify the relevant information, such as the purpose of the code and the requirements it must meet, before they can begin to evaluate the code itself.

Situated Learning Theory: Situated Learning Theory emphasizes the importance of learning in context. In code review, this means that reviewers must understand the context in which the code was written, such as the requirements of the project and the programming language used, in order to effectively evaluate the code.

Learning by Teaching Theory: Learning by Teaching Theory suggests that individuals can improve their own learning by teaching others. In code review, this means that developers can improve their own skills and knowledge by reviewing the code of others and providing feedback. Through this process, they can gain a deeper understanding of programming concepts and best practices.

By understanding these theories and applying them to code review in software development, teams can improve their code quality, promote learning and collaboration among team members, and ultimately deliver better software.

\subsection*{What theories can we use for understanding onboarding in software development}

Onboarding is a critical process in software development that involves integrating new team members into an existing team, providing them with the information and resources they need to be successful, and helping them become productive as quickly as possible. Here are some theories that can be used to understand onboarding in software development:

Socialization Theory: Socialization Theory emphasizes the importance of socialization in helping new team members become integrated into an existing team. In onboarding, this means that organizations should focus on creating opportunities for new team members to interact with existing team members, such as through mentorship programs, team-building exercises, and social events.

Self-Determination Theory: Self-Determination Theory suggests that individuals are motivated by three basic needs: autonomy, competence, and relatedness. In onboarding, this means that organizations should focus on providing new team members with opportunities to develop their skills and expertise, as well as providing them with a sense of belonging and connection to the team.

Expectancy Theory: Expectancy Theory suggests that individuals are motivated by their expectations of how their efforts will lead to desired outcomes. In onboarding, this means that organizations should provide new team members with a clear understanding of what is expected of them and what they can expect in terms of feedback, support, and recognition.

Information Processing Theory: Information Processing Theory suggests that humans process information in stages, starting with sensory input and moving through various levels of processing before generating a response. In onboarding, this means that organizations should provide new team members with the information and resources they need to be successful, and help them to understand how their work fits into the larger goals of the organization.

Goal Setting Theory: Goal Setting Theory suggests that individuals are more motivated when they have clear goals and objectives to work towards. In onboarding, this means that organizations should work with new team members to set clear goals and expectations, and provide them with the support and resources they need to achieve those goals.

By understanding these theories and applying them to onboarding in software development, organizations can help new team members become integrated and productive more quickly, improve retention rates, and ultimately improve the quality of their software development.

\subsection*{What theories can we use for understanding automated program repair in software development}

Automated program repair (APR) is an emerging field in software engineering that focuses on developing techniques to automatically fix defects in software code. Here are some theories that can be used to understand APR in software development:

Search-Based Software Engineering (SBSE) Theory: SBSE theory emphasizes the use of search algorithms to solve problems in software engineering. In APR, this means that algorithms are used to search for solutions to defects in software code. The search algorithms can be guided by various criteria, such as program correctness, code readability, and program performance.

Machine Learning Theory: Machine Learning Theory suggests that machines can learn from data and use that learning to make predictions and decisions. In APR, this means that machine learning techniques can be used to analyze software code and identify defects, and to learn from previous repair attempts to improve the effectiveness of future repairs.

Evolutionary Computation Theory: Evolutionary Computation Theory is a subfield of SBSE that focuses on using algorithms inspired by biological evolution to solve optimization problems. In APR, this means that evolutionary algorithms can be used to evolve a set of program repairs over time, with the fittest solutions surviving and being used to guide future repairs.

Human-Computer Interaction (HCI) Theory: HCI Theory emphasizes the importance of designing systems that are usable and effective for humans. In APR, this means that the design of APR systems should consider the needs of human users, such as software developers and users of the software.

Fault Localization Theory: Fault Localization Theory focuses on identifying the source of faults in software code. In APR, this means that techniques for identifying the location and nature of software defects can be used to guide the search for solutions to those defects.

By understanding these theories and applying them to APR in software development, researchers and practitioners can improve the effectiveness and efficiency of automated program repair techniques, ultimately improving the quality of software code and reducing development costs.

\subsection*{What theories from psychology can we use for understanding the impact of automated debugging in software development?}

Automated debugging is a process that involves the use of software tools to identify and diagnose defects in software code. Here are some theories from psychology that can be used to understand the impact of automated debugging in software development:

Cognitive Load Theory: Cognitive Load Theory suggests that humans have a limited amount of cognitive resources available for processing information. In automated debugging, this means that tools that reduce the cognitive load required to diagnose defects, such as automated bug detection and suggestion systems, can improve the productivity and effectiveness of developers.

Attention Restoration Theory: Attention Restoration Theory suggests that exposure to natural environments and other restorative environments can help restore cognitive function and reduce mental fatigue. In automated debugging, this means that tools that provide developers with restorative breaks or reduce the cognitive demands of debugging can improve the effectiveness of developers.

Expectancy Theory: Expectancy Theory suggests that individuals are motivated by their expectations of how their efforts will lead to desired outcomes. In automated debugging, this means that tools that provide developers with clear feedback on the results of their debugging efforts, such as the effectiveness of a proposed fix, can improve the motivation and effectiveness of developers.

Goal Setting Theory: Goal Setting Theory suggests that individuals are more motivated when they have clear goals and objectives to work towards. In automated debugging, this means that tools that help developers to set clear goals and prioritize their debugging efforts, such as by suggesting the most critical defects to address, can improve the motivation and effectiveness of developers.

Social Learning Theory: Social Learning Theory suggests that individuals learn by observing the behavior of others and the consequences of that behavior. In automated debugging, this means that tools that allow developers to learn from the debugging efforts of others, such as through collaborative debugging or access to a knowledge base of previously fixed defects, can improve the effectiveness of developers.

By understanding these theories and applying them to automated debugging in software development, researchers and practitioners can improve the effectiveness of automated debugging tools, ultimately improving the quality of software code and reducing development costs.
